# Supplementary material for: Joint 3D Human Shape Recovery and Pose Estimation from a Single Image with Bilayer Graph
Source: arXiv:2110.08472 source file (2021-12-05)
Supplement: Supplementary file 1 [file supplemental.tex]

\section*{Additional Studies and Results}
\label{sec:supplementary}

% \subsection*{Errata}

% We would like to briefly address a few omissions in our paper submission. Please note that we do not introduce any new information, but merely aim to clarify a few items.

% In Section 3 we refer to graph linear layers. A graph linear layer has identity adjacency matrix, and thus only operate on the features of each node in the graph~\cite{kolotouros2019cmr}.

% There are some omissions in Section 4.5

% \begin{itemize}
%     % \item \textbf{Section 4.5} Table 2, the row labeled F should say ``Post W.Share FL". \textbf{Or not?}

%     \item \textbf{Study 5} We omitted to state ``compare row D with row H".
    
%     \item \textbf{Study 6} (False) and (True), rows K and L in Table 2, mean without and with weight sharing.
    
%     \item \textbf{Study 7} The ``2" refers to Table 2, and ``No.I" refers to the row labeled I in Table 2.
% \end{itemize}

\subsection*{Per-Activity Evaluation for Human 3.6M}

The Human 3.6M dataset~\cite{h36m_pami, IonescuSminchisescu11} contains people performing 15 activities, such as sitting down and walking. In the main paper, we reported our best model as shown in Table~\textcolor{red}{2}, which apply No Weight Sharing, Pre\_Fusion and focal loss with parameters set to \(A=1\), \(B=5\) and \(\gamma=1\). Table~\ref{tbl:per_activity_results} shows the evaluation on Human 3.6M for each activity separately. The activities represent Providing Directions, Having a Discussion, Eating, Greeting, Making a Phone Call, Taking a Photo, Posing, Making a Purchase, Sitting, Sitting Down, Smoking, Waiting, Walking a Dog, Walking Together, and Walking respectively. It is clear from the table that the performance for certain activities (highlighted in blue), .e.g, Walking, compares favorably to others, e.g. Sitting Down (highlighted in red), as those poses are more challenging and consequently have higher errors.

%{\HC where ... }
% \Note{JVB: I've changed red and blue, since red is usually associated with failure, error, etc. and blue (or green) tend be used for success, or improvement, etc.}

\begin{table*}[thb!]
\centering
% \tiny
% \scriptsize
\begin{tabular}{l | c | c | c | c | c | c | c | c}
  \hline
   \multicolumn{1}{l|}{} & \multicolumn{4}{|c|}{H36M P1} & \multicolumn{4}{|c}{H36M P2} \\
  \hline
     \multirow{2}{*}{Act.} & MPJPE & RE & MPJPE & RE & MPJPE & RE & MPJPE & RE \\
     & (np) & (np) & (p) & (p) & (np) & (np) & (p) & (p) \\
  \hline
     %A & G-CMR~\cite{kolotouros2019cmr} & 75.0 & 51.2 & 74.7 & 51.9 & 72.7 & 49.3  & 71.9 & 50.1 & - & - & 91.46 & 88.6 9& 0.87 & 0.66  \\
\textcolor{blue}{Direct}& 59.32&   32.34&   61.28&   35.41 & \textbf{52.12}&   \textbf{28.27}&   \textbf{55.43}&   \textbf{31.76} \\
Discus & 59.68&   35.37&   62.77&   38.55 & 56.46&   35.06&   61.09&   37.98 \\
Eat & 59.50&   34.78&   62.34&   37.63 & 53.81&   31.86&   57.29&   35.94  \\
Greet & 69.62&   42.56&   70.35&   44.48 & 66.70&   42.13&   67.54&   43.27  \\
Phone & 59.81&   35.99&   64.21&   40.34 & 55.35&   33.36&   60.57&   38.27 \\
Photo & 66.76&   39.66&   72.08&   45.54 & 61.80&   38.83&   68.33&   44.55 \\
\textcolor{blue}{Posing}& 59.88&   33.53&   62.42&   39.06 & 57.72&   31.50&   59.42&   36.67  \\
Purch & 61.18&   34.42&   66.51&   38.01 & 60.29&   33.24&   68.18&   38.65 \\
\textcolor{red}{Sit}& 69.01&   43.22&   74.01&   47.12 & 67.76&   44.03&   73.37&   48.37  \\
\textcolor{red}{SitDn}& 81.00&   56.64&   85.55&   58.32 & 85.64&   58.51&   93.59&   62.33\\
Smoke & 58.14&   36.14&   62.16&   40.55 & 53.14&   33.42&   59.00&   38.59  \\
Wait& 65.97&   40.84&   67.44&   42.61 & 63.84&   39.72&   64.43&   40.78 \\
WlkD & 58.77&   37.32&   64.99&   40.80 & 59.64&   38.74&   65.44&   41.95 \\
\textcolor{blue}{WlkT} & 56.89&   32.19&   59.88&   36.39 & 56.60&   31.58&   59.52&   35.90 \\
\textcolor{blue}{Wlk} & \textbf{53.27} & \textbf{30.00} & \textbf{56.09} & \textbf{33.33} & 53.45&   29.60&   56.01&   32.79  \\
\hdashline
Overall& 62.38&   37.69&   65.91&   41.22 & 59.73&   36.57&   64.10&   40.41  \\
  \hline
\end{tabular}
\vspace*{5pt}
\caption{Evaluation results on Human 3.6M per activity. Certain activities (highlighted in blue) result in better performance, compared to others (highlighted in red). Some poses are more challenging and consequently have higher errors.}
\label{tbl:per_activity_results}
\end{table*}

\subsection*{Learning Performance}

Figure~\ref{fig:eval_ckp} shows a plot of the training loss for our best model (see the paper submission, Table 1 - Ours and Table 2 - row E). Our model achieves a lower loss much earlier compared to the Graph CMR~\cite{kolotouros2019cmr} baseline. This suggest that we can reduce the number of epochs for which we train the models. Especially, the loss of the proposed model is more stable than the the baseline, whose curve oscillates less than it.

%Another interesting observation in ~\ref{fig:eval_ckp} is that 

Table~\ref{tbl:eval_ckp} shows the evaluation results at different checkpoints during training. A checkpoint refers to saving the trainable weights of the entire model to file after a certain number of steps. We store many such checkpoints for each training run. One epoch takes about 5,000 steps. After training for 26 epochs (130,000 steps), the performance only slightly improves (See Tables 1 and 2 row E in our submission paper).

\begin{table*}[thb!]
\centering
\scriptsize
\begin{tabular}{l | c | c | c | c | c | c | c | c | c | c | c | c | c | c }
  \hline
   & \multicolumn{4}{|c|}{H36M P1} & \multicolumn{4}{|c|}{H36M P2} & \multicolumn{2}{|c|}{UP-3D} & \multicolumn{4}{|c}{LSP} \\
  \hline
     \multirow{2}{*}{}{Epoch} & MPJPE & RE & MPJPE & RE & MPJPE & RE & MPJPE & RE & Sh. Err. & Sh. Err. & \multirow{2}{*}{FB Acc.} & \multirow{2}{*}{FB F1} & \multirow{2}{*}{Parts Acc.} & \multirow{2}{*}{Parts F1} \\
     (Step) & (np) & (np) & (p) & (p) & (np) & (np) & (p) & (p) & (np) & (p) & & & & \\
%  \hline
%    Methods & \multicolumn{7}{c}{} \\
  \hline
2 (10k) &79.12& 50.16& 91.06& 57.66&  78.11& 51.72& 88.17& 58.94&  103.59& 95.58&  89.02& 0.81& 87.21& 0.59\\
4 (20k) &67.87& 44.79& 76.10& 50.73&  66.82& 45.29& 73.73& 50.43&  90.06& 92.05 &  91.17& 0.86& 89.13& 0.67\\
6 (30k) &74.15& 43.82& 79.85& 48.83&  74.30& 44.05& 77.09& 47.82&  83.61& 79.12 &  91.41& 0.86& 89.26& 0.68\\
8 (40k) &68.86& 42.28& 72.12& 46.34&  69.21& 42.66& 72.34& 46.10& 80.74& 79.27  & 92.13 & 0.88& 89.94& 0.70\\
14 (70k) &  66.16& 40.75& 68.01& 43.97& 63.93& 40.66& 66.09& 43.63& 75.28& 74.03& 92.02& 0.87& 90.01& 0.70 \\
20 (100k) & 67.43& 40.07& 68.63& 43.34& 64.14& 38.55& 66.28& 41.21& 70.48& 69.20& 92.61& 0.89& 90.35& 0.72 \\
26 (130K) & 64.02& 38.44& 66.79& 41.94& 60.81& 37.29& 64.00& 40.91& 69.11& 69.04& 92.53& 0.88& 90.45& 0.72 \\

  \hline
\end{tabular}
\vspace*{5pt}
\caption{Results for evaluation of checkpoints on Human 3.6M, LSP and UP-3D datasets. The checkpoints are saved when training on the mixed datasets for 50 epochs. Please note that one epoch takes about 5,000 steps. The rows show both MSE and L1 los.  Error metrics MPJPE and RE are defined in~\cite{Zhou:2019:MMHM}. The Shape errors are MSE losses between the estimated shape and ground truth SMPL shape. For evaluation datasets H36M P1, P2 and UP-3D the errors metrics are reported for non-parametric (np) and parametric SMPL meshes (p). For LSP evaluation we report accuracy and F1 score. After 26 epochs the improvement compared to our best model (See Tables 1 and 2 row E in our submission paper).
%\Note{JVB: What is the meaning of 2, 4, 6 and 8 in the table? Are they different checkpoints, or what?}
}
\label{tbl:eval_ckp}
\end{table*}

\begin{figure}[th!]
\centering
    \subfigure[3D Keypoints Loss]{%
        \label{fig:first}%
        \includegraphics[width=0.5\linewidth]{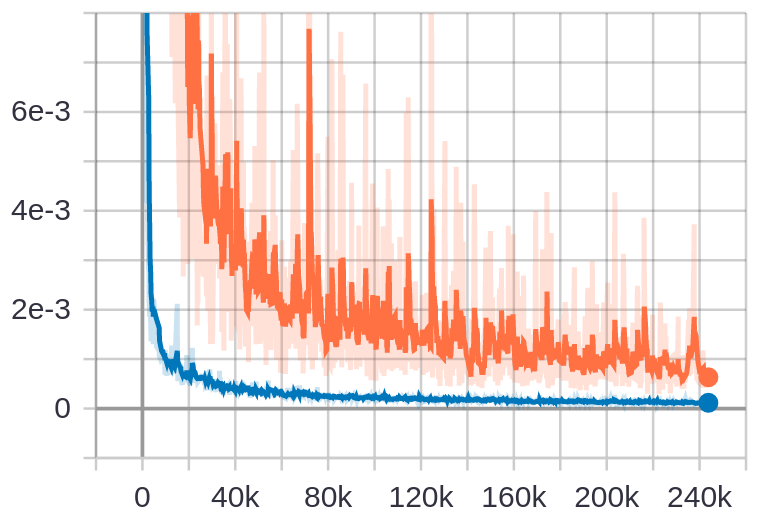}}%
    \subfigure[Shape Loss]{%
        \label{fig:second}%
        \includegraphics[width=0.5\linewidth]{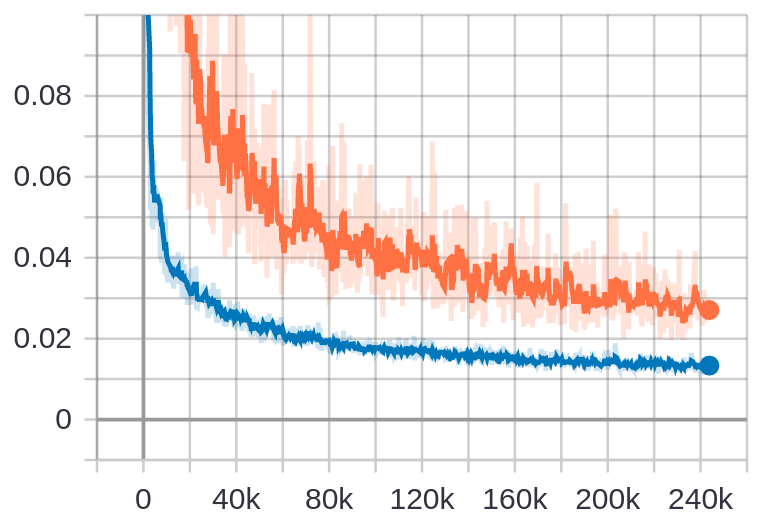}}%
    % \begin{subfigure}[t]{0.5\textwidth}
    %     \centering
    %     \includegraphics[width=0.45\linewidth]{images/loss_kp_3d_fixed.png}
    %     \caption{The 3D Keypoints loss during training epochs. Orange = Graph CMR, Blue = Ours}
    % \end{subfigure}
    % \qquad
    % \begin{subfigure}[t]{0.5\textwidth}
    %     \centering
    %     \includegraphics[width=0.45\linewidth]{images/loss_shape_fixed.png} 
    %     \caption{The Shape loss during training epochs. Orange = Graph CMR, Blue = Ours}
    % \end{subfigure}
    \caption{Comparison of the 3D Keypoints and Shape loss between the baseline (Orange) and our proposed model (Blue). We trained for 50 epochs and one epoch takes about 5,000 steps. The X axes are MSE loss (in meter) and L1 loss (in meter) respectively in~\ref{fig:first} and~\ref{fig:second}. Please note that we optimize 3D keypoint Focal Loss instead of MSE loss when training the proposed model and we plot MSE loss here to compare with the baseline.}
    \label{fig:eval_ckp}
\end{figure}

% \begin{itemize}
%     \item Show that our method tends to ``converge" faster.
%     \item Show results for different training checkpoints.
% \end{itemize}

\subsection*{Focal Loss}

\begin{figure}[ht!]
\centering
    \includegraphics[width=0.9\linewidth]{images/focal_loss_New.pdf}
    \caption{Focal loss plots for different parameter values. We also plot \(L_1\) and \(L_2\) for comparison.}
    \label{fig:focal_loss}
\end{figure}

We defined a version of focal loss for the regression of joints and meshes in Section 3.5 as:

\begin{align}
\nonumber
    \mathcal{L}_{fl} = -B (A \cdot \mathcal{L}_{L_1})^{\gamma} \log(1-A \cdot \mathcal{L}_{L_1}).
\end{align}

Figure~\ref{fig:focal_loss} shows plots of our focal loss formulation for different values of \(A, B\) and \(\gamma\).

\subsection*{Qualitative Results}

As described in Section 4, and shown in Tables 1 and 2, we evaluate our model on various datasets. Figure~\ref{fig:qualitative_results_h36m_up3d} shows examples of qualitative results for the evaluation images from the UP-3D and Human 3.6M datasets.

\begin{figure*}[th!]
    \centering
    \includegraphics[width=0.88\textwidth]{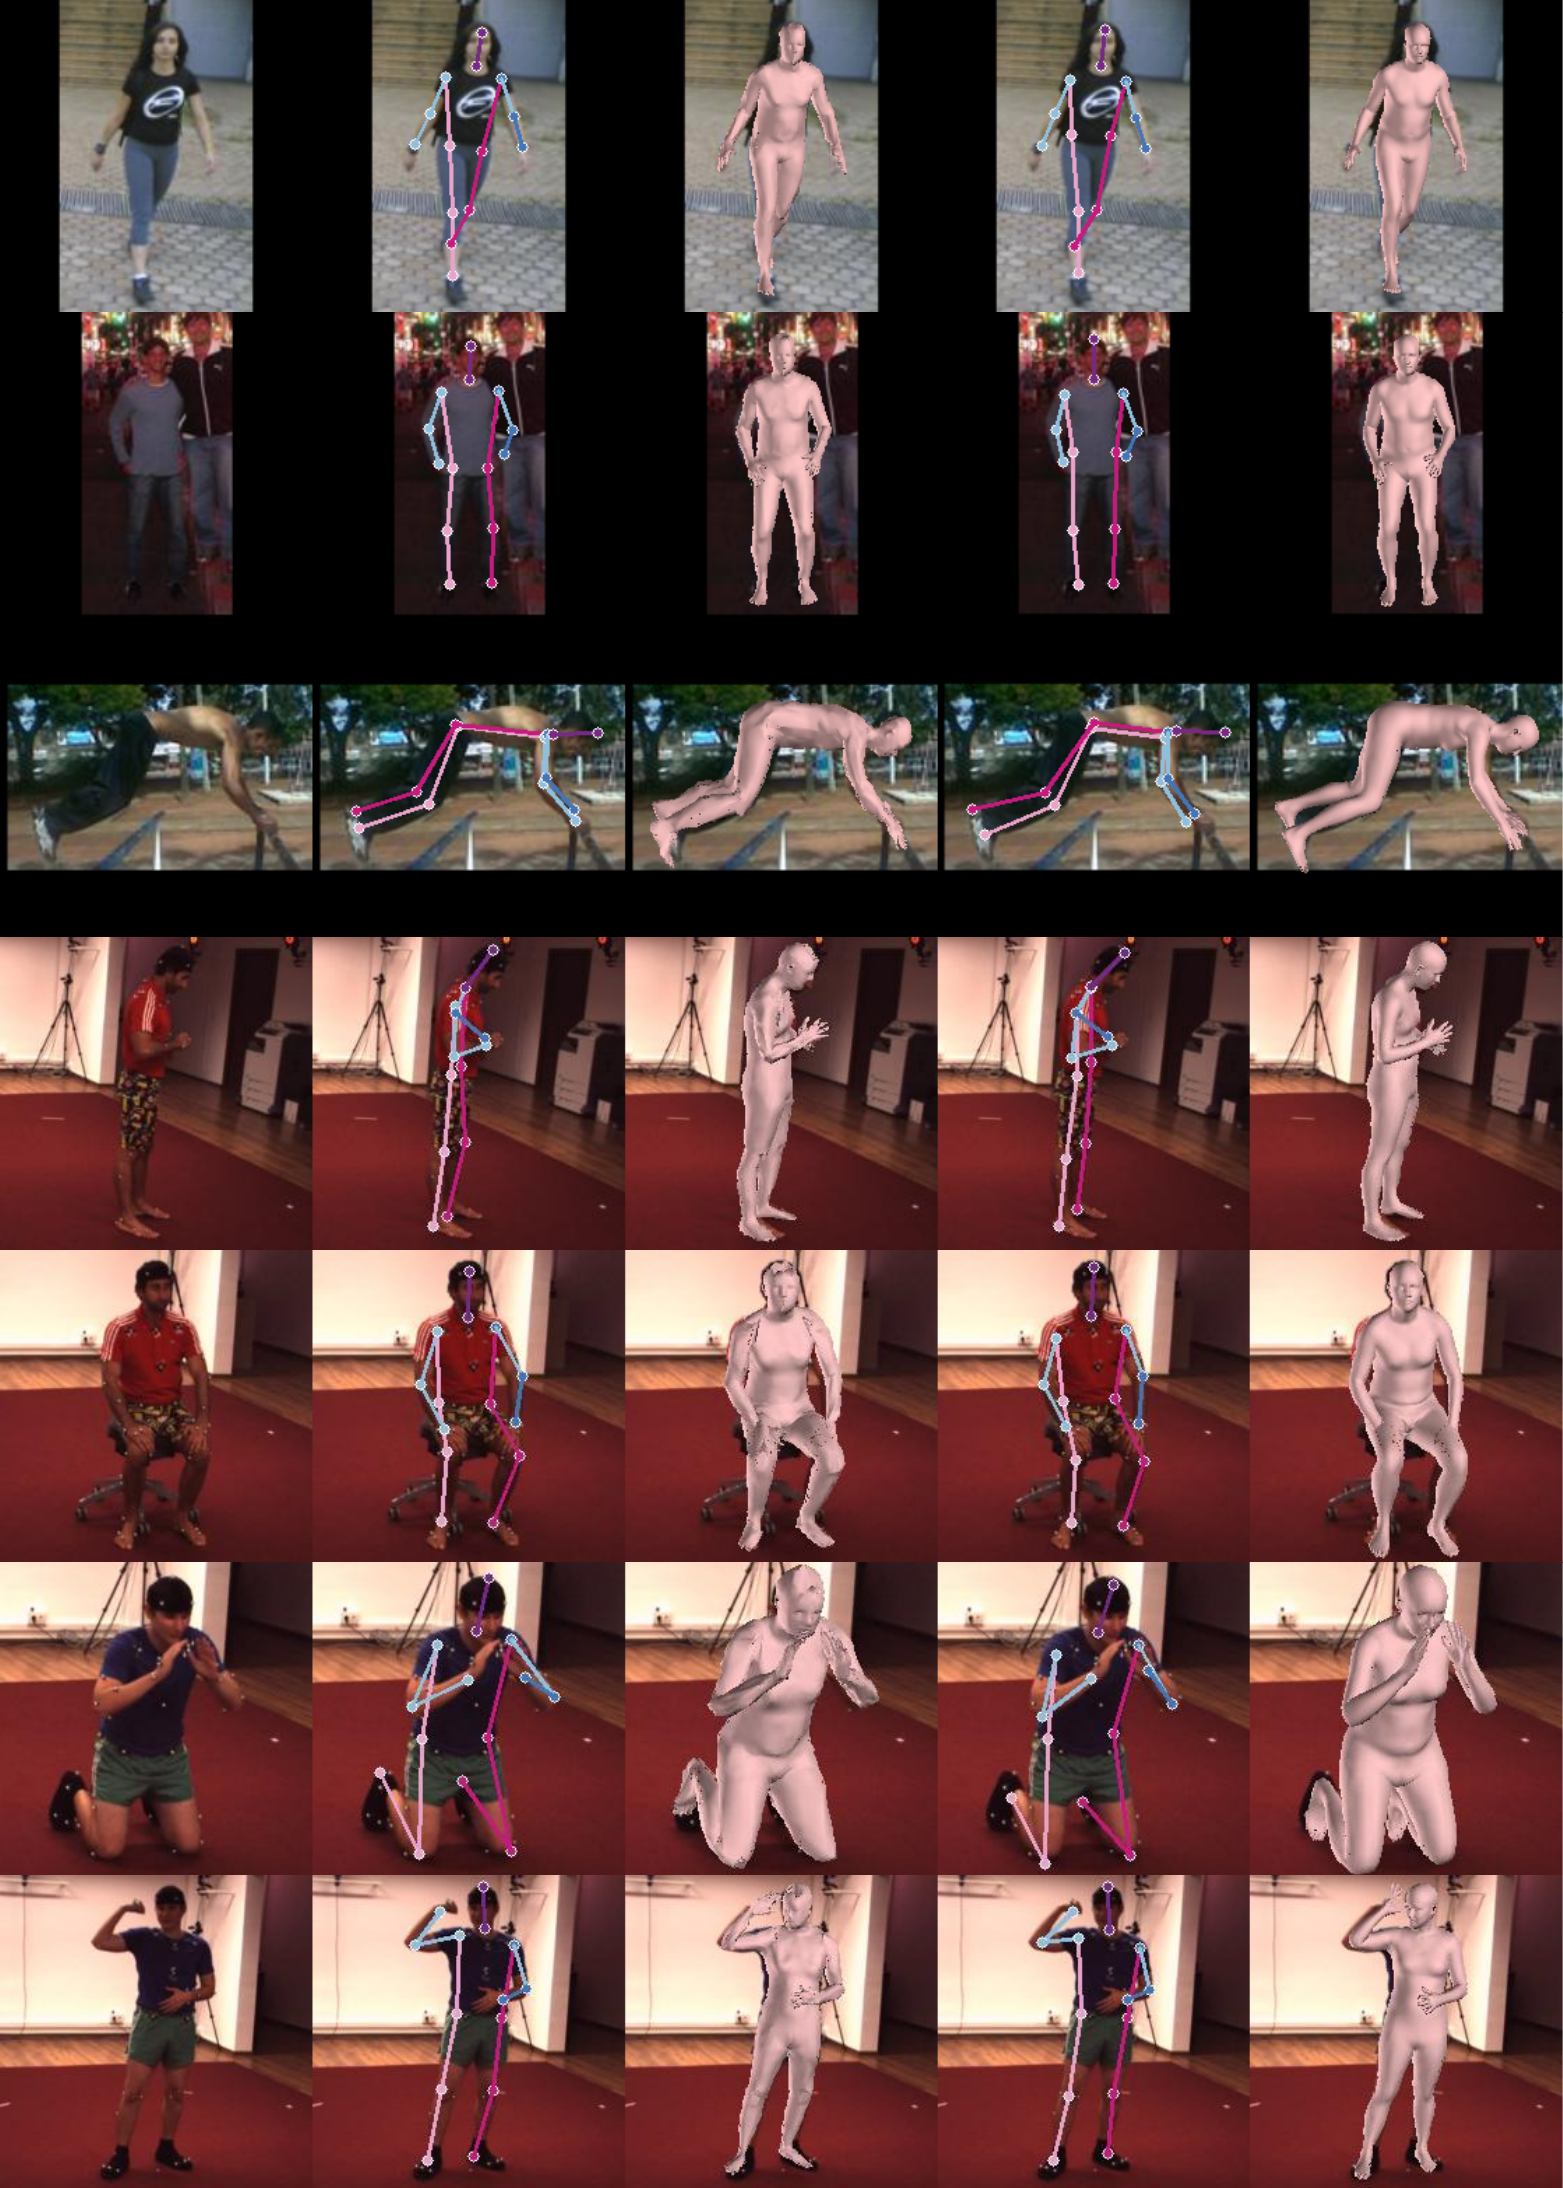}
    \caption{Qualitative results. From left to right: original input image, non-parametric pose and shape, parametric pose and shape. The first three rows are examples from UP-3D. The remaining rows are examples from Human 3.6M, for actors 9 and 11.}
    \label{fig:qualitative_results_h36m_up3d}
\end{figure*}

\subsection*{Additional Ablation Study}

\textcolor{blue}{
Removed from the main paper:
\textbf{Study 5} All the experiments annotated with FL in ~\ref{tbl:ablation_results} apply the focal loss with \(A=1\) , \(B=5\) and \(\gamma = 1\). We have explored values for \(B\) in the range 5 to 10 and the performances are roughly the same. To determine the influence of the focal loss to the performance, we train our models with focal loss where \(B = 5\) and without focal loss. Compare rows D and H. Table~\ref{tbl:ablation_results} shows that the focal loss can help boost performance. As a regression task with dense prediction, the focal loss will more substantially penalize joints or vertices with large loss. The small ratio of bad predictions will not be ignored even if most predictions are good. It further improves the performance of our multi-scale architecture.\\
\textbf{Study 7} We also explore some methods to solve the instability problem caused by the last ReLU in the prediction of camera parameters (see Sec.~\ref{subsec:training}). Both Replacing it with LeakyReLU and applying BatchNorm instead works well. In Table~\ref{tbl:ablation_results} all the experiments use BatchNorm, except for row I which uses LeakyReLU.
}
No.I-J explore global features to feed into the joint mesh. Please note that No.I is the same as in Table 2 in the submission paper and is shown here for better comparison. All the three models apply the same settings as No.E in Table 2 of the main paper: Pre\_fusion without weight sharing  and 3D keypoints focal loss with $A=1, B=5, \gamma=1$. It is clear that global feature is too coarse to recover an accurate 3D shape. BatchNorm in the camera layers is important to avoid bad camera prediction. The model performance can be unstable without it as shown in No.I of Table~\ref{tbl:more_ablation_results}. 

No.O-P also apply Pre\_fusion and use $A=1, B=10, \gamma=1$ as the 3D keypoints focal loss instead. $B=10$ still performs well although slightly inferior to $B=5$ when comparing with No.E and No.D in Table 2 in the submission paper.

\begin{table*}[thb!]
\centering
\tiny
\begin{tabular}{l | l | c | c | c | c | c | c | c | c | c | c | c | c | c | c }
  \hline
   \multicolumn{2}{l|}{} & \multicolumn{4}{|c|}{H36M P1} & \multicolumn{4}{|c|}{H36M P2} & \multicolumn{2}{|c|}{UP-3D} & \multicolumn{4}{|c}{LSP} \\
  \hline
     \multirow{2}{*}{No.} & \multirow{2}{*}{Methods} & MPJPE & RE & MPJPE & RE & MPJPE & RE & MPJPE & RE & Sh. Err. & Sh. Err. & \multirow{2}{*}{FB Acc.} & \multirow{2}{*}{FB F1} & \multirow{2}{*}{Parts Acc.} & \multirow{2}{*}{Parts F1} \\
     & & (np) & (np) & (p) & (p) & (np) & (np) & (p) & (p) & (np) & (p) & & & & \\
  \hline

J & gFeat FL    &                   91.80 & 60.03 & 93.55 & 62.34 & 90.23 & 57.95 & 93.01 & 60.82 & 115.56 & 115.17 & 90.67 & 0.85 & 88.00 & 0.64 \\
M & gFeat BN FL &                   72.75& 48.77& 71.63& 49.97& 68.08& 46.22& 66.77& 47.52& 96.31&  96.64& 91.91& 0.87& 89.44& 0.68 \\
N & gFeat BN    &                   74.23& 52.27& 74.60& 53.51& 69.22& 49.36& 69.68& 50.85& 99.90& 101.25& 91.60& 0.87& 89.18& 0.68 \\
O & B=10(False) &                   65.07& 39.02& 72.07& 42.35& 61.91& 38.05& 69.46& 41.37& 71.74&  71.86& 92.25& 0.88& 90.16& 0.71 \\
P & B=10(True)  &                   62.67& 43.09& 65.64& 46.97& 63.05& 43.23& 64.95& 45.76& 89.21&  86.34& 92.30& 0.88& 90.15& 0.71 \\

  \hline
\end{tabular}
\vspace*{5pt}
\caption{Evaluation results for additional ablation studies of using global features, and $B=10$. gFeat represents global feature, FL is for focal loss, BN is for batch norm inserted after ReLU of the first camera layer. True/False in the last two rows indicate the model share or not share weights between joint branch and mesh branch.}
\label{tbl:more_ablation_results}
\end{table*}

\subsection*{Non-Parametric vs Parametric}

As shown in Figure~\ref{fig:qualitative_results_h36m_up3d} and Figure 5 in our submission paper, the shape of the parametric (SMPL) prediction is smooth and the shape of the non-parametric prediction can have some small artifacts. However, the non-parametric shape is the regression result of all vertices in the mesh and is thus able to learn the pose better (see MPJPE and RE metrics in Table 1,2 and Table~\ref{tbl:more_ablation_results}). Regressing the parameters for the SMPL shape reconstruction is prone to introduce some errors. The reason for this is that the SMPL shapes cannot represent some of the deformations for certain poses of the humans. For example, we can observe that some keypoints of the SMPL prediction are slightly off the ground truth in the last two rows of Figure~\ref{fig:qualitative_results_h36m_up3d}. Due to its dense prediction, the non-parametric methods, e.g. our proposed multi-scale GCN, is promising to produce a more accurate 3D reconstruction. To avoid some of the noise or artifacts, we can apply some surface constraints, like vertex normal loss, to smooth the predicted surface for non-parametric methods in the future.
